# Supplementary material for: Mo' States Mo' Problems: Emergency Stop Mechanisms from Observation
Source: arXiv:1912.01649 source file (2019-12-03)
Supplement: Supplementary file 1 [file lowerbounds.tex]

\section{Lower bounds} \label{app:lower}
We provide a corresponding lower bound to examine the tightness of \cref{lem:cover}.
\begin{lemma}
There exists an MDP $M$, distance $d$ and expert state distribution support $\mathcal{S}_{\rho_{\expertpolicy}}$ such that
\begin{multline}
    \mathbb{P}\left( \bigcap_{s \in \mathcal{S}_{\expertpolicy}} \min_{s' \in D} d(s, s') \leq \delta_d \right) = 1 - |\mathcal{S}_{\expertpolicy}| ( 1 - \epsilon_d)^n  \\ + {|\mathcal{S}_{\expertpolicy}| \choose 2}(1 - 2\epsilon_d)^n - {|\mathcal{S}_{\expertpolicy}| \choose 3}(1 - 3\epsilon_d)^n  + \dotsc
\end{multline}
\end{lemma}
In other words, this shows \cref{lem:cover} is tight up to at least the first two terms.
\begin{proof}   
Consider an MDP $M$ where $|\mathcal{S}_{\expertpolicy}| = \frac{1}{\epsilon_d}$, $\rho_{\expertpolicy}^t$ is uniform and $d(s, s') > \delta_d \; \forall s \neq s'$. The proof follows from \cref{lem:dice}
\begin{align}
    \mathbb{P}\left( \bigcap_{s \in \mathcal{S}_{\expertpolicy}} \min_{s' \in D} d(s, s') \leq \delta_d \right) &= 1 - \mathbb{P}\left( \bigcup_{s \in \mathcal{S}_{\expertpolicy}} \min_{s' \in D} d(s, s') \geq \delta_d \right) \\
    &= 1 - \mathbb{P}\left( \bigcup_{s \in \mathcal{S}_{\expertpolicy}} s \neq s' \; \forall s' \in D \right) \\
    &= 1 - {|\mathcal{S}_{\expertpolicy}| \choose 1} ( 1 - \epsilon_d)^n + {|\mathcal{S}_{\expertpolicy}| \choose 2}(1 - 2\epsilon_d)^n - {|\mathcal{S}_{\expertpolicy}| \choose 3}(1 - 3\epsilon_d)^n  + \dotsc
\end{align}
\end{proof}

\begin{lemma} \label{lem:dice}
% From https://math.stackexchange.com/questions/266505/a-number-of-dice-rolls-to-see-every-number-at-least-once
% Remember to cite this!
Consider randomly sampling with replacement $n$ times from a set of $m$ equally probable events $A_1, \dotsc, A_m$. The probability of at least one of each event occurring is equal to
\begin{equation}
    1 - {m \choose 1}\left(1 - \frac{1}{m}\right)^n + {m \choose 2}\left(1 - \frac{2}{m}\right)^n - {m \choose 3}\left(1 - \frac{3}{m}\right)^n
\end{equation}
\end{lemma}
\begin{proof}
Let $B_k$ denote the set of outcomes where event $A_k$ does not occur during the $n$ samples. By application of the inclusion-exclusion principle, the number of outcomes where at least one event does not occur is
\begin{align}
    \left| \bigcup_{k=1}^m B_k \right| &= \sum_{k=1}^m | B_k| - \sum_{j < k} |B_j \cap B_k| + \sum_{i < j < k} |B_i \cap B_j \cap B-k| - \dotsc \\
    &= {m \choose 1}(m - 1)^n - {m \choose 2}(m - 2)^n + {m \choose 3}(m - 3)^n - \dotsc
\end{align}
Thus, the probability that all events occur is
\begin{gather}
    \frac{m^n - {m \choose 1}(m - 1)^n + {m \choose 2}(m - 2)^n - {m \choose 3}(m - 3)^n - \dotsc}{m^n} \\
    1 - {m \choose 1}\left(1 - \frac{1}{m}\right)^n + {m \choose 2}\left(1 - \frac{2}{m}\right)^n - {m \choose 3}\left(1 - \frac{3}{m}\right)^n
\end{gather}
\end{proof}
